# Supplementary material for: Nonlinear features of the superconductor--ferromagnet--superconductor $\varphi_0$ Josephson junction in ferromagnetic resonance region
Source: arXiv:2210.00366 source file (2022-10-01)
Supplement: Supplementary file 1 [file shukrinov_supplementary.pdf]

# Supplementary materials for "Nonlinear features of the superconductor–ferromagnet–superconductor $\varphi_0$ Josephson junction in ferromagnetic resonance region"

Aliasghar Janalizadeh[1], Ilhom R. Rahmonov[2,3,4], Sara A. Abdelmoneim [5], Yury M. Shukrinov[2,3,4], and Mohammad R. Kolahchi[1]

[1] *Department of Physics, Institute for Advanced Studies in Basic Sciences (IASBS), P.O. Box 45137-66731, Zanjan, Iran*
[2] *BLTP, JINR, Dubna, Moscow Region, 141980, Russia*
[3] *Dubna State University, Dubna, 141980, Russia*
[4] *Moscow Institute of Physics and Technology, Dolgoprudny, 141700, Moscow Region, Russia*
[5] *Physics department, Menofiya University, Faculty of Science, 32511, Shebin Elkom,Egypt*
(Dated: October 1, 2022)

According to our approximation, at small system parameters the $y$ component of magnetization can be determined by the general Duffing equation (1):

$$\frac{d^2m_y}{dt^2} + 2\alpha\omega_F\frac{dm_y}{dt} + \omega_F^2 m_y - \omega_F^2 m_y^3 = \omega_F^2 Gr\sin(\omega_J t).(1)$$

In Eq.(1) the $\alpha$ is a phenomenological damping constant, $\omega_F$ is the frequency of the ferromagnetic resonance, $\omega_J$ is the Josephson frequency, $G$ is the ratio of the Josephson to the magnetic energy and parameter $r$ determines by the strength of the spin-orbit interaction.

In order to find frequency response function for equation (1) we have performed the following procedure. We assume that the approximation solution of equation (1) has a form

$$m_y = a\sin\omega_J t + b\cos\omega_J t, \qquad (2)$$

where $a$ and $b$ are the function of $\omega_J$.

First and second order derivatives of $m_y$ are determined by

$$\frac{dm_y}{dt} = a\omega_J\cos\omega_J t - b\omega_J\sin\omega_J t \qquad (3)$$
$$\frac{d^2m_y}{dt^2} = -a\omega_J^2\sin\omega_J t - b\omega_J^2\cos\omega_J t$$

Using the trigonometric identities the cube of $m_y$ can be written as

$$m_y^3 = \frac{3}{4}(a^2+b^2)[a\sin\omega_J t + b\cos\omega_J t] \qquad (4)$$

Substituting (3) and (4) into the equation (1) and equating coefficients at $\sin\omega_J t$ and $\cos\omega_J t$ we find

$$[\omega_F^2 - \omega_J^2 - \frac{3}{4}\omega_F^2(m_y^{max})^2]a - 2\alpha\omega_F\omega_J b = \omega_F^2 Gr$$
$$2\alpha\omega_F\omega_J a + [\omega_F^2 - \omega_J^2 - \frac{3}{4}\omega_F^2(m_y^{max})^2]b = 0 \qquad (5)$$

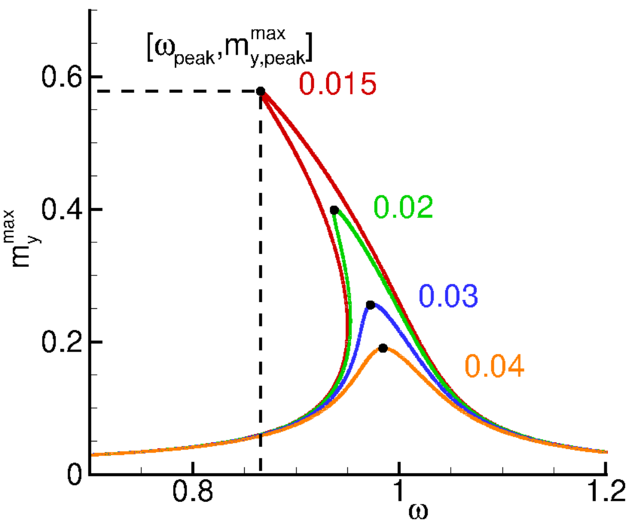


Figure 1. Frequency response Eq.7, i.e. $m_y^{max}$ versus $\omega$ for $G = 0.05$, $r = 0.05$ and $\omega_F = 0.5$. Here numbers indicate the value of $\alpha$.

where $(m_y^{max})^2 = a^2 + b^2$. Squaring both side of system of equations (5) and by summation them, we get the frequency response function

$$(m_y^{max})^2 = \frac{\left(\omega_F^2 Gr\right)^2}{\left[\omega_J^2 - \omega_F^2 + \frac{3}{4}\omega_F^2(m_y^{max})^2\right]^2 + \left(2\alpha\omega_F\omega_J\right)^2}(6)$$

Introducing the $\omega = \omega_J/\omega_F$ we can rewrite it in a simple form

$$(m_y^{max})^2 = \frac{\left(Gr\right)^2}{\left[\omega^2 - 1 + \frac{3}{4}(m_y^{max})^2\right]^2 + \left(2\alpha\omega\right)^2} \qquad (7)$$

In Fig.1 the frequency dependence of the amplitude corresponding to the expression (7) for values of $\alpha = 0.015, 0.02, 0.03, 0.04$ are demonstrated.

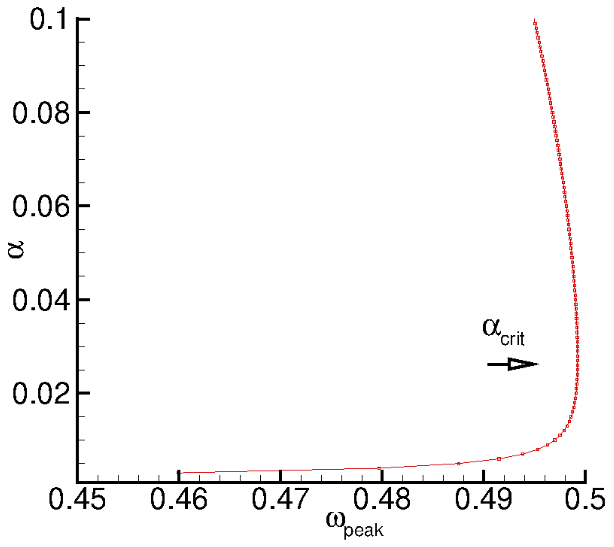


Figure 2. The resonance peak position depending on $\alpha$ for $G = 0.05$ and $r = 0.05$ and $\omega_F = 0.5$.

To find the analytical anomalous damping dependence, we need to differentiate both side of expression (7) with respect to $\omega$ and equate $d(m_y^{max})/d\omega$ to zero. As the result, we find

$$(m_{y,peak}^{max})^2 = \frac{4}{3}(1 - \omega_{peak}^2 - 2\alpha^2). \quad (8)$$

Here $m_{y,peak}^{max}$ is the resonance peak and $\omega_{peak}$ is its position as shown in Fig.??. Finally, substituting (8) into (7), we obtain

$$\frac{4}{3}(1 - \omega_{peak}^2 - 2\alpha^2) = \frac{(Gr)^2}{(-2\alpha^2)^2 + (2\alpha\omega_{peak})^2} \quad (9)$$

and after simplification of this expression, it can be written as

$$\frac{16}{3}\alpha^2(\alpha^2 + \omega_{peak}^2 - 3\alpha^2\omega_{peak}^2 - \omega_{peak}^4 - 2\alpha^4) = (Gr)^2. \quad (10)$$

The solution of equation (10) with respest to $\omega$ has the form

$$\omega_{peak} = \sqrt{\frac{1 - 3\alpha^2}{2} + \frac{1}{2}\sqrt{(1 - \alpha^2)^2 - 12(\frac{Gr}{4\alpha})^2}} \quad (11)$$

So, it is analytical expression for ADD and its plot is shown in Fig.2 for $G = 0.05$ and $r = 0.05$.

We can also find the expression for critical $\alpha$. To get it, we perform following procedure. After taking the derivative of expression (10) with respect to the $\alpha$ we are equating $\partial\omega_{peak}/\partial\alpha$ to zero we obtain the expression for $\alpha_{crit}$

$$6\alpha_{crit}^4 - 2\alpha_{crit}^2(1 - 3\omega_{peak}^2) - \omega_{peak}^2 + \omega_{peak}^4 = 0 \quad (12)$$

Substituting $\omega_{peak}$ in (12) from (11), we get

$$9\left(\frac{Gr}{4\alpha_{crit}}\right)^4 + 3\alpha_{crit}^2(10\alpha_{crit}^2 - 1)\left(\frac{Gr}{4\alpha_{crit}}\right)^2 - 2\alpha_{crit}^4(\alpha_{crit}^2 - 1)^2 = 0 \quad (13)$$

Taking into account $10\alpha_{crit}^2 << 1$ and $\alpha_{crit}^2 << 1$, the equation (13) can be rewritten as

$$9\left(\frac{Gr}{4\alpha_{crit}}\right)^4 - 3\alpha_{crit}^2\left(\frac{Gr}{4\alpha_{crit}}\right)^2 - 2\alpha_{crit}^4 = 0 \quad (14)$$

Solution of (14) has a form

$$\left(\frac{Gr}{4\alpha_{crit}}\right)^2 = \frac{3\alpha_{crit}^2 \pm \sqrt{9\alpha_{crit}^4 + 72\alpha_{crit}^4}}{18} \quad (15)$$

or

$$\left(\frac{Gr}{4\alpha_{crit}}\right)^2 = \frac{\alpha_{crit}^2 \pm 3\alpha_{crit}^2}{6} \quad (16)$$

From here we can find

$$\alpha_{crit} = \frac{1}{2}\sqrt{\sqrt{\frac{3}{2}}Gr}. \quad (17)$$
